# Supplementary material for: Nonlocal Thermoelectricity in a S-TI-S Junction in Contact with a N-Metal Probe: Evidence for Helical Edge States
Source: arXiv:1911.04367 source file (2020-06-03)
Supplement: Supplementary file 1 [file supplementary_ArXiv_2.pdf]

## SUPPLEMENTARY MATERIAL

# Nonlocal Thermoelectricity in a Superconductor–Topological-Insulator–Superconductor Junction in Contact with a Normal-Metal Probe: Evidence for Helical Edge States


Gianmichele Blasi,[1,*] Fabio Taddei,[1] Liliana Arrachea,[2] Matteo Carrega,[1] and Alessandro Braggio[1,†]

[1] *NEST, Scuola Normale Superiore and Instituto Nanoscienze-CNR, I-56126, Pisa, Italy*

[2] *International Center for Advanced Studies, ECyT-UNSAM, Campus Miguelete, 25 de Mayo y Francia, 1650 Buenos Aires, Argentina*


## SCATTERING MATRIX

Here, we determine the full scattering matrix of the setup depicted in Fig. 1($a$) of the main text. We start by considering the scattering problem associated to the topological Josephson junction, evaluating the scattering matrix coefficients at the interface between superconducting leads ($\mathrm{S_L}/\mathrm{S_R}$) and the upper edge state of the TI. In order to do that, we first consider the case of an incident spin-up electron, incoming from the TI towards the interface with the right superconductor $\mathrm{S_R}$. The incoming wave reflects back into the TI region in a left-moving spin-down electron or a left-moving spin-down hole; while into the superconducting region it transmits (if the energy is not in the gap) as a right-moving spin-up electron-like or a right-moving spin-up hole-like quasi-particle:

$$\Psi^{TI}_{e_+}(x_0^-) + r^R_{ee}\Psi^{TI}_{e_-}(x_0^-) + r^R_{he}\Psi^{TI}_{h_-}(x_0^-) = t^R_{\tilde{e}e}\Psi^{S_R,j}_{e_+}(x_0^+) + t^R_{\tilde{h}e}\Psi^{S_R,j}_{h_+}(x_0^+) \tag{S.1}$$

In that case $x_0^\pm = \lim_{\delta\to 0^\pm} x_0 + \delta$ with $x_0 = L/2$. Similar equations can be found for incoming holes, QPs and QHs at both the interfaces. In Eq. ($S.1$) (and similar) $\Psi^{TI}_{e_\pm}$ and $\Psi^{TI}_{h_\pm}$ represent the right/left-moving electrons/holes eigenfuctions in the $TI$; while $\Psi^{i,j}_{e_\pm}$ and $\Psi^{i,j}_{h_\pm}$ represent the right/left-moving QPs/QHs eigenfuctions in the $i = \mathrm{S_L}, \mathrm{S_R}$ superconductor (as reported in Eq. (2) of the main text), with $j = \mathrm{sign}(\epsilon - |\Delta - |\epsilon_{DS}||)$. The coefficients $r^{\mathrm{L/R}}_{\alpha,\beta}$ and $t^{\mathrm{L/R}}_{\alpha,\beta}$ represent respectively the reflection and transmission amplitudes of an incoming particle of type $\beta$ to a particle of type $\alpha$ at the left/right interface. Here we indicate with $\{\alpha,\beta\} = \{e,h\}$ electrons and holes in the $TI$ and with $\{\alpha,\beta\} = \{\tilde{e},\tilde{h}\}$ QPs and QHs in the superconductors.

In order to find the solutions for the scattering amplitudes of Eqs. ($S.1$) we have to impose the boundary condition obtained by integrating the BdG equation (see Eq. 1 in the main text):

$$\begin{cases} -\lambda^* u_\uparrow(x_0^-) = -\lambda u_\uparrow(x_0^+) \\ \lambda u_\downarrow(x_0^-) = \lambda^* u_\downarrow(x_0^+) \\ -\lambda v_\uparrow(x_0^-) = -\lambda^* v_\uparrow(x_0^+) \\ \lambda^* v_\downarrow(x_0^-) = \lambda v_\downarrow(x_0^+) \end{cases} \tag{S.2}$$

where $\lambda = 1 + i\frac{\Lambda}{2\hbar v_F}$ and $x_0 = \pm\frac{L}{2}$. The explicit solution of the linear set of equations (Eq. ($S.1$) and similar) with the boundary conditions of Eq. ($S.2$), leads to the following scattering amplitudes for the left

$$x_0 = -\frac{L}{2} \quad \begin{cases} r^L_{he} = -\frac{v_+}{u_+}e^{i\alpha_+}e^{-i\phi_L} & t^L_{\tilde{e}e} = -\frac{\lambda^*}{\lambda}\frac{\sqrt{u_+^2 - v_+^2}}{u_+}e^{\frac{i}{2}(\alpha_+ - \beta_+)}e^{-i\frac{\phi_L}{2}}\cdot\Theta(|\epsilon_+| - \Delta) \\ r^L_{eh} = \frac{v_-}{u_-}e^{i\alpha_-}e^{i\phi_L} & t^L_{\tilde{h}h} = \frac{\lambda}{\lambda^*}\frac{\sqrt{u_-^2 - v_-^2}}{u_-}e^{\frac{i}{2}(\alpha_- - \beta_-)}e^{i\frac{\phi_L}{2}}\cdot\Theta(|\epsilon_-| - \Delta) \\ r^L_{h\tilde{e}} = -\frac{v_-}{u_-}e^{-i\beta_-}\cdot\Theta(|\epsilon_-| - \Delta) & t^L_{e\tilde{e}} = \frac{\lambda^*}{\lambda}\frac{\sqrt{u_-^2 - v_-^2}}{u_-}e^{\frac{i}{2}(\alpha_- - \beta_-)}e^{i\frac{\phi_L}{2}}\cdot\Theta(|\epsilon_-| - \Delta) \\ r^L_{e\tilde{h}} = -\frac{v_+}{u_+}e^{-i\beta_+}\cdot\Theta(|\epsilon_+| - \Delta) & t^L_{h\tilde{h}} = \frac{\lambda}{\lambda^*}\frac{\sqrt{u_+^2 - v_+^2}}{u_+}e^{\frac{i}{2}(\alpha_+ - \beta_+)}e^{-i\frac{\phi_L}{2}}\cdot\Theta(|\epsilon_+| - \Delta) \end{cases}$$

and the right interface

$$x_0 = \frac{L}{2} \quad \begin{cases} r^R_{he} = \frac{v_-}{u_-} e^{i\alpha_-} e^{-i\phi_R} & t^R_{\tilde{e}e} = \frac{\lambda^*}{\lambda} \frac{\sqrt{u_-^2 - v_-^2}}{u_-} e^{\frac{i}{2}(\alpha_- - \beta_-)} e^{-i\frac{\phi_R}{2}} \cdot \Theta(|\epsilon_-| - \Delta) \\ r^R_{eh} = -\frac{v_+}{u_+} e^{i\alpha_+} e^{i\phi_R} & t^R_{\tilde{h}h} = \frac{\lambda}{\lambda^*} \frac{\sqrt{u_+^2 - v_+^2}}{u_+} e^{\frac{i}{2}(\alpha_+ - \beta_+)} e^{i\frac{\phi_R}{2}} \cdot \Theta(|\epsilon_+| - \Delta) \\ r^R_{\tilde{h}\tilde{e}} = -\frac{v_+}{u_+} e^{-i\beta_+} \cdot \Theta(|\epsilon_+| - \Delta) & t^R_{e\tilde{e}} = -\frac{\lambda^*}{\lambda} \frac{\sqrt{u_+^2 - v_+^2}}{u_+} e^{\frac{i}{2}(\alpha_+ - \beta_+)} e^{i\frac{\phi_R}{2}} \cdot \Theta(|\epsilon_+| - \Delta) \\ r^R_{\tilde{e}\tilde{h}} = -\frac{v_-}{u_-} e^{-i\beta_-} \cdot \Theta(|\epsilon_-| - \Delta) & t^R_{h\tilde{h}} = \frac{\lambda}{\lambda^*} \frac{\sqrt{u_-^2 - v_-^2}}{u_-} e^{\frac{i}{2}(\alpha_- - \beta_-)} e^{-i\frac{\phi_R}{2}} \cdot \Theta(|\epsilon_-| - \Delta) \end{cases}$$

While, when $|\epsilon_{DS}| > \Delta$, for $0 < \epsilon < |\Delta - |\epsilon_{DS}||$, hold the following relations for the left

$$x_0 = -\frac{L}{2} \quad \begin{cases} r^L_{he} = -\frac{v_+}{u_+} e^{i\alpha_+} e^{-i\phi_L} & t^L_{\tilde{e}e} = -\frac{\lambda^*}{\lambda} \frac{\sqrt{u_+^2 - v_+^2}}{u_+} e^{\frac{i}{2}(\alpha_+ - \beta_+)} e^{-i\frac{\phi_L}{2}} \\ r^L_{eh} = -\frac{v_-}{u_-} e^{i\alpha_-} e^{i\phi_L} & t^L_{\tilde{h}h} = \frac{\lambda}{\lambda^*} \frac{\sqrt{u_-^2 - v_-^2}}{u_-} e^{\frac{i}{2}(\alpha_- + \beta_-)} e^{i\frac{\phi_L}{2}} \\ r^L_{\tilde{h}\tilde{e}} = -\frac{v_-}{u_-} e^{i\beta_-} & t^L_{e\tilde{e}} = -\frac{\lambda^*}{\lambda} \frac{\sqrt{u_-^2 - v_-^2}}{u_-} e^{\frac{i}{2}(\alpha_- + \beta_-)} e^{i\frac{\phi_L}{2}} \\ r^L_{\tilde{e}\tilde{h}} = -\frac{v_+}{u_+} e^{-i\beta_+} & t^L_{h\tilde{h}} = \frac{\lambda}{\lambda^*} \frac{\sqrt{u_+^2 - v_+^2}}{u_+} e^{\frac{i}{2}(\alpha_+ - \beta_+)} e^{-i\frac{\phi_L}{2}} \end{cases}$$

and the right interface

$$x_0 = \frac{L}{2} \quad \begin{cases} r^R_{he} = -\frac{v_-}{u_-} e^{i\alpha_-} e^{-i\phi_R} & t^R_{\tilde{e}e} = -\frac{\lambda^*}{\lambda} \frac{\sqrt{u_-^2 - v_-^2}}{u_-} e^{\frac{i}{2}(\alpha_- + \beta_-)} e^{-i\frac{\phi_R}{2}} \\ r^R_{eh} = -\frac{v_+}{u_+} e^{i\alpha_+} e^{i\phi_R} & t^R_{\tilde{h}h} = \frac{\lambda}{\lambda^*} \frac{\sqrt{u_+^2 - v_+^2}}{u_+} e^{\frac{i}{2}(\alpha_+ - \beta_+)} e^{i\frac{\phi_R}{2}} \\ r^R_{\tilde{h}\tilde{e}} = -\frac{v_+}{u_+} e^{-i\beta_+} & t^R_{e\tilde{e}} = -\frac{\lambda^*}{\lambda} \frac{\sqrt{u_+^2 - v_+^2}}{u_+} e^{\frac{i}{2}(\alpha_+ - \beta_+)} e^{i\frac{\phi_R}{2}} \\ r^R_{\tilde{e}\tilde{h}} = -\frac{v_-}{u_-} e^{i\beta_-} & t^R_{h\tilde{h}} = \frac{\lambda}{\lambda^*} \frac{\sqrt{u_-^2 - v_-^2}}{u_-} e^{\frac{i}{2}(\alpha_- + \beta_-)} e^{-i\frac{\phi_R}{2}} \end{cases}$$

in which

$$\alpha_\pm = \frac{\epsilon \pm \epsilon_{DS}}{\epsilon_c}; \qquad \beta_\pm = \frac{\sqrt{(\epsilon \pm \epsilon_{DS})^2 - \Delta^2}}{\epsilon_c} \tag{S.3}$$

with $\epsilon_c = \frac{\hbar v_F}{L}$ is the confining energy. In the above expressions we focused on positive energies $\epsilon \geq 0$ since in the expression of the currents (reported in Eq. (S.9)) the integration is performed over $\epsilon \in [0, \infty[$. Now, we consider the full system with the normal probe tunnel coupled to the upper edge of the TI. The full scattering matrix in Nambu space is

$$\Psi^\alpha_{(i,a)}|_{out} = S^{\alpha\beta}_{(i,a)(j,b)} \Psi^{\beta\eta}_{(j,b)}|_{in} \tag{S.4}$$

between incoming/outgoing states $(j,b)/(i,a)$ with $\{a,b\} = \{\uparrow,\downarrow\}$ labeling the spin-channel at the respective lead $i,j = \mathrm{N}, \mathrm{S_L}, \mathrm{S_R}$. In Eq. (S.4), $\{\alpha,\beta\} = \{e,h\}$ indicate electrons and holes in the normal probe $N$, while $\{\alpha,\beta\} = \{\tilde{e},\tilde{h}\}$ label QPs and QHs in the superconductors. In particular we assume a symmetric beam splitter which describes the

contact interface between the normal lead N and the TI. The beam splitter is characterized by a reflection and transmission amplitudes

$$r = \cos(\eta) \quad \text{and} \quad t = i\ \sin(\eta) \tag{S.5}$$

which depend on only one parameter $\eta \in \left[0, \frac{\pi}{2}\right]$, such that $|r|^2 + |t|^2 = 1$ (as required by unitarity). In order to keep the presentation simple, here we preferred not to specifically discuss any energy dependency of the coupling amplitude $t$. In fact, if this was the case, the actual value of the nonlocal thermoelectric current would depend on the details of the function $t(E)$ which has non universal nature. Nevertheless, also in this case, the main result of the paper would remain unchanged, i. e. the purely non-local thermoelectric effect is a unique signature of the helical nature of the edge states.

By taking into account the scattering amplitudes at the interfaces with the superconductors obtained above we get the full scattering matrix of the system:

$$\begin{pmatrix} c_N^{\downarrow} \\ c_N^{\uparrow} \\ c_{\mathrm{S_L}}^{\downarrow} \\ c_{\mathrm{S_R}}^{\uparrow} \\ b_N^{\downarrow} \\ b_N^{\uparrow} \\ b_{\mathrm{S_L}}^{\downarrow} \\ b_{\mathrm{S_R}}^{\uparrow} \end{pmatrix}_{out} = \begin{pmatrix} 0 & a_2 & 0 & a_4 & C_1 & 0 & C_3 & 0 \\ a_1 & 0 & a_3 & 0 & 0 & C_2 & 0 & C_4 \\ 0 & b_2 & 0 & b_4 & D_1 & 0 & D_3 & 0 \\ b_1 & 0 & b_3 & 0 & 0 & D_2 & 0 & D_4 \\ A_1 & 0 & A_3 & 0 & 0 & c_2 & 0 & c_4 \\ 0 & A_2 & 0 & A_4 & c_1 & 0 & c_3 & 0 \\ B_1 & 0 & B_3 & 0 & 0 & d_2 & 0 & d_4 \\ 0 & B_2 & 0 & B_4 & d_1 & 0 & d_3 & 0 \end{pmatrix}_S \begin{pmatrix} c_N^{\uparrow} \\ c_N^{\downarrow} \\ c_{\mathrm{S_L}}^{\uparrow} \\ c_{\mathrm{S_R}}^{\downarrow} \\ b_N^{\uparrow} \\ b_N^{\downarrow} \\ b_{\mathrm{S_L}}^{\uparrow} \\ b_{\mathrm{S_R}}^{\downarrow} \end{pmatrix}_{in} \tag{S.6}$$

where

$$\begin{aligned}
&a_1 = r + \tfrac{r^L_{eh} r^R_{he} t^2 r^*}{1-r^L_{eh} r^R_{he}|r|^2}; \quad a_2 = \tfrac{r^R_{eh} r^L_{he} t^2 r^*}{1-r^R_{eh} r^L_{he}|r|^2} + r; \quad a_3 = \tfrac{t t^L_{e\tilde{e}}}{1-r^L_{eh} r^R_{he}|r|^2}; \quad a_4 = \tfrac{t t^R_{e\tilde{e}}}{1-r^R_{eh} r^L_{he}|r|^2};\\
&b_1 = \tfrac{t t^R_{\tilde{e}e}}{1-r^L_{eh} r^R_{he}|r|^2}; \quad b_2 = \tfrac{t t^L_{\tilde{e}e}}{1-r^R_{eh} r^L_{he}|r|^2}; \quad b_3 = \tfrac{r t^L_{e\tilde{e}} t^R_{\tilde{e}e}}{1-r^L_{eh} r^R_{he}|r|^2}; \quad b_4 = \tfrac{r t^L_{\tilde{e}e} t^R_{e\tilde{e}}}{1-r^R_{eh} r^L_{he}|r|^2};\\
&c_1 = r^* + \tfrac{r r^R_{eh} r^L_{he} \left(t^2\right)^*}{1-r^R_{eh} r^L_{he}|r|^2}; \quad c_2 = r^* + \tfrac{r r^L_{eh} r^R_{he} \left(t^2\right)^*}{1-r^L_{eh} r^R_{he}|r|^2}; \quad c_3 = \tfrac{t^L_{h\tilde{h}} t^*}{1-r^R_{eh} r^L_{he}|r|^2}; \quad c_4 = \tfrac{t^R_{h\tilde{h}} t^*}{1-r^L_{eh} r^R_{he}|r|^2};\\
&d_1 = \tfrac{t^R_{\tilde{h}h} t^*}{1-r^R_{eh} r^L_{he}|r|^2}; \quad d_2 = \tfrac{t^L_{\tilde{h}h} t^*}{1-r^L_{eh} r^R_{he}|r|^2}; \quad d_3 = \tfrac{t^L_{h\tilde{h}} t^R_{\tilde{h}h} r^*}{1-r^L_{eh} r^R_{he}|r|^2}; \quad d_4 = \tfrac{t^L_{Hh} t^R_{hH} r^*}{1-r^L_{eh} r^R_{he}|r|^2};\\
&A_1 = \tfrac{r^R_{he}|t|^2}{1-r^L_{eh} r^R_{he}|r|^2}; \quad A_2 = \tfrac{r^L_{he}|t|^2}{1-r^L_{eh} r^R_{he}|r|^2}; \quad A_3 = \tfrac{r r^R_{he} t^L_{e\tilde{e}} t^*}{1-r^L_{eh} r^R_{he}|r|^2}; \quad A_4 = \tfrac{r r^L_{he} t^R_{e\tilde{e}} t^*}{1-r^L_{eh} r^R_{he}|r|^2};\\
&B_1 = \tfrac{r^R_{he} t t^L_{\tilde{h}h} r^*}{1-r^L_{eh} r^R_{he}|r|^2}; \quad B_2 = \tfrac{r^L_{he} t t^R_{\tilde{h}h} r^*}{1-r^L_{eh} r^R_{he}|r|^2}; \quad B_3 = r^L_{\tilde{h}\tilde{e}} + \tfrac{r^R_{he} t^L_{e\tilde{e}} t^L_{\tilde{h}h}|r|^2}{1-r^L_{eh} r^R_{he}|r|^2}; \quad B_4 = r^R_{\tilde{h}\tilde{e}} + \tfrac{r^L_{he} t^R_{e\tilde{e}} t^R_{\tilde{h}h}|r|^2}{1-r^L_{eh} r^R_{he}|r|^2};\\
&C_1 = \tfrac{r^R_{eh}|t|^2}{1-r^L_{eh} r^R_{he}|r|^2}; \quad C_2 = \tfrac{r^L_{eh}|t|^2}{1-r^L_{eh} r^R_{he}|r|^2}; \quad C_3 = \tfrac{r^R_{eh} t t^L_{h\tilde{h}} r^*}{1-r^L_{eh} r^R_{he}|r|^2}; \quad C_4 = \tfrac{r^L_{eh} t t^R_{h\tilde{h}} r^*}{1-r^L_{eh} r^R_{he}|r|^2};\\
&D_1 = \tfrac{r r^R_{eh} t^L_{\tilde{e}e} t^*}{1-r^L_{eh} r^R_{he}|r|^2}; \quad D_2 = \tfrac{r r^L_{eh} t^R_{\tilde{e}e} t^*}{1-r^L_{eh} r^R_{he}|r|^2}; \quad D_3 = r^L_{\tilde{e}\tilde{h}} + \tfrac{r^R_{eh} t^L_{\tilde{e}e} t^L_{h\tilde{h}}|r|^2}{1-r^L_{eh} r^R_{he}|r|^2}; \quad D_4 = r^R_{\tilde{e}\tilde{h}} + \tfrac{r^L_{eh} t^R_{\tilde{e}e} t^R_{h\tilde{h}}|r|^2}{1-r^L_{eh} r^R_{he}|r|^2}.
\end{aligned} \tag{S.7}$$

In Eq. (S.6) we have indicated with $c_i^{\uparrow\downarrow}$ and $b_i^{\uparrow\downarrow}$ the incoming and outgoing electrons and hole respectively with $i = \mathrm{S_L}, \mathrm{S_R}, \mathrm{N}$ labelling the corresponding lead. As an example of the derivation of the non-zero entries of the scattering matrix, let us explicit the calculation of the term $a_1$, which relates an incoming spin-up electron with an outgoing spin-up electron at the same $N$ metallic lead

$$\begin{aligned}
c^{\uparrow}_{N+} \rightarrow c^{\uparrow}_{N-} :& \\
a_1 &= r + t r^R_{he} r^* r^L_{eh} t + t r^R_{he} r^* r^L_{eh} r r^R_{he} r^* r^L_{eh} t + \dots \\
&= r + t^2 r^R_{he} r^* r^L_{eh} \sum_{n=0}^{\infty} \left( r^L_{eh} r^R_{he} \, |r|^2 \right)^n \\
&= r + \frac{r^L_{eh} r^R_{he} t^2 r^*}{1 - r^L_{eh} r^R_{he} \, |r|^2}
\end{aligned} \tag{S.8}$$

## EVALUATION OF CURRENTS

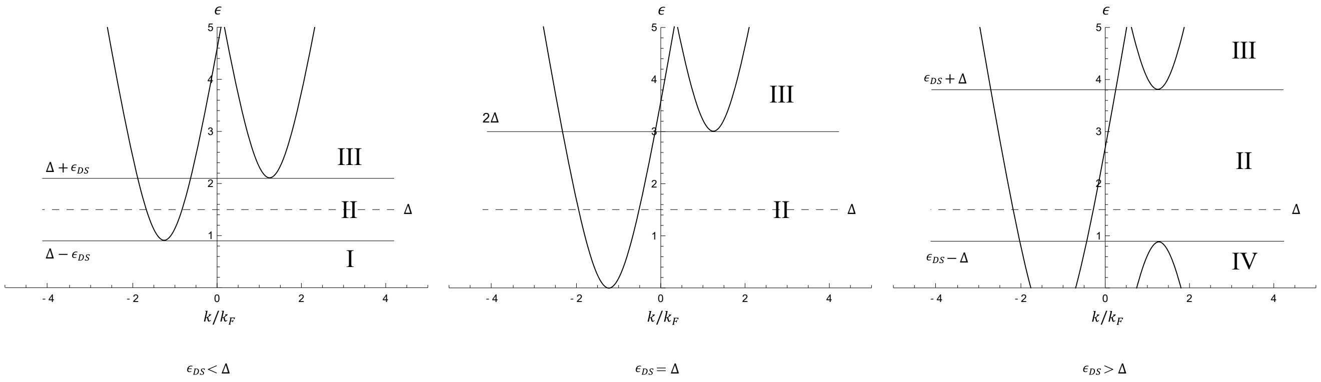


Figure 1: Regions of integration in Eq. (S.11) for $\epsilon_{DS} > 0$: $\epsilon_{DS} < \Delta$ (left panel), $\epsilon_{DS} = \Delta$ (middle panel), $\epsilon_{DS} > \Delta$ (right panel).

As already mentioned in the main text (see Eq. (3)), the charge and heat currents can be written as [5]

$$J_i^k = \frac{2}{h}\sum_j \sum_{\alpha,\beta} (\alpha e)^{1-k} \int_0^\infty d\epsilon\ (\epsilon - \mu_i)^k \times \left(f_i^\alpha(\epsilon) - f_j^\beta(\epsilon)\right) P_{i,j}^{\alpha,\beta}(\epsilon), \tag{S.9}$$

where the scattering coefficients $P_{i,j}^{\alpha,\beta}$ are defined as the trace over the channels $\{a,b\} = \{\uparrow,\downarrow\}$ of the scattering matrix introduced in Eq. *S*.4 and computed in Eqs. *S*.6 and *S*.7

$$P_{i,j}^{\alpha,\beta}(\epsilon,\phi,\Phi) = \sum_{a,b} \left| S_{(i,a),(j,b)}^{\alpha,\beta} \right|^2, \tag{S.10}$$

where we have made explicit the dependence on the phase difference $\phi$ and the flux bias $\Phi$. Notice that $P_{i,j}$ satisfies the time-reversal symmetry relations, namely $P_{i,j}^{\alpha,\beta}(\epsilon,\phi,\Phi) = P_{j,i}^{\beta,\alpha}(\epsilon,-\phi,-\Phi)$ [5]. Finally Eq. (*S*.9) can be conveniently recast as follows

$$J_i^k = \frac{2e^{(1-k)}}{h}\left(\int_I j_{i,I}^k d\epsilon + \int_{II} j_{i,II}^k d\epsilon + \int_{III} j_{i,III}^k d\epsilon + \int_{IV} j_{i,IV}^k d\epsilon\right) \tag{S.11}$$

where integrals are performed over the energy regions $I$, $II$, $III$ and $IV$ depicted in Fig. 1, which represent, respectively, the contributions deriving from the sub-gap (region I), the semi-continuum (region II) and the full continuum (regions III and IV). The full analytical expressions of the current integrands of Eq. (*S*.11) have been calculated, leading to some straightforward but cumbersome expressions that we do not report here for brevity.

## CHARGE CURRENT AND ROLE OF THE PROBE'S TEMPERATURE

We can compute analytically the probe charge current $J_N^0$ of Eqs. (*S*.11) in the lowest order in $t$, i.e. keeping the leading term in $|t|^2$. This represents a situation in which the probe is weakly coupled with the system and can be conveniently compared with the results computed with other methods such as the tunneling approach (see later). The analytical expressions for the integrands of Eqs. (*S*.11) in this regime are given by:

$$j_{N,I}^0 = \mathcal{O}(|t|^4) \tag{S.12}$$

$$j^0_{N,II}=\left\{\left(f^+_N(\epsilon)-f^-_N(\epsilon)\right)\left[\frac{\left(e^{4\cosh^{-1}\left(\frac{|\epsilon_{DS}|+\epsilon}{\Delta}\right)}-1\right)}{-2e^{2\cosh^{-1}\left(\frac{|\epsilon_{DS}|+\epsilon}{\Delta}\right)}\cos\left(\frac{2\epsilon_{DS}}{\epsilon_C}+\frac{2L(\epsilon_{DS}+\mathrm{sgn}(\epsilon_{DS})\epsilon)}{\Delta}-\mathrm{sgn}(\epsilon_{DS})\phi\right)+e^{4\cosh^{-1}\left(\frac{|\epsilon_{DS}|+\epsilon}{\Delta}\right)}+1}\right]+\right.$$
$$-\left(f^+_{\mathrm{S_R}}(\epsilon)-f^-_{\mathrm{S_L}}(\epsilon)\right)\frac{\left(e^{2\cosh^{-1}\left(\frac{\epsilon_{DS}+\epsilon}{\Delta}\right)}-1\right)^2}{-2e^{2\cosh^{-1}\left(\frac{\epsilon_{DS}+\epsilon}{\Delta}\right)}\cos\left(\frac{2\epsilon_{DS}}{\epsilon_C}+\frac{2L(\epsilon_{DS}+\epsilon)}{\Delta}+\phi\right)+e^{4\cosh^{-1}\left(\frac{\epsilon_{DS}+\epsilon}{\Delta}\right)}+1}\Theta(\epsilon_{DS})$$
$$\left.-\left(f^+_{\mathrm{S_L}}(\epsilon)-f^-_{\mathrm{S_R}}(\epsilon)\right)\frac{\left(e^{2\cosh^{-1}\left(\frac{-\epsilon_{DS}+\epsilon}{\Delta}\right)}-1\right)^2}{-2e^{2\cosh^{-1}\left(\frac{-\epsilon_{DS}+\epsilon}{\Delta}\right)}\cos\left(\frac{2\epsilon_{DS}}{\epsilon_C}-\frac{2L(-\epsilon_{DS}+\epsilon)}{\Delta}+\phi\right)+e^{4\cosh^{-1}\left(\frac{-\epsilon_{DS}+\epsilon}{\Delta}\right)}+1}\Theta(-\epsilon_{DS})\right\}|t|^2+\mathcal{O}(|t|^4) \tag{S.13}$$

$$j^0_{N,III}=\left[\left(f^+_N(\epsilon)-f^-_N(\epsilon)\right)\left(\frac{2\left(e^{2\cosh^{-1}\left(\frac{\epsilon-\epsilon_{DS}}{\Delta}\right)}\cos\left(-\frac{2\epsilon_{DS}}{\epsilon_C}+\frac{2L(\epsilon-\epsilon_{DS})}{\Delta}-\phi\right)-1\right)}{-2e^{2\cosh^{-1}\left(\frac{\epsilon-\epsilon_{DS}}{\Delta}\right)}\cos\left(-\frac{2\epsilon_{DS}}{\epsilon_C}+\frac{2L(\epsilon-\epsilon_{DS})}{\Delta}-\phi\right)+e^{4\cosh^{-1}\left(\frac{\epsilon-\epsilon_{DS}}{\Delta}\right)}+1}+\right.\right.$$
$$\left.+\frac{2\left(e^{2\cosh^{-1}\left(\frac{\epsilon_{DS}+\epsilon}{\Delta}\right)}\cos\left(\frac{2\epsilon_{DS}}{\epsilon_C}+\frac{2L(\epsilon_{DS}+\epsilon)}{\Delta}+\phi\right)-1\right)}{-2e^{2\cosh^{-1}\left(\frac{\epsilon_{DS}+\epsilon}{\Delta}\right)}\cos\left(\frac{2\epsilon_{DS}}{\epsilon_C}+\frac{2L(\epsilon_{DS}+\epsilon)}{\Delta}+\phi\right)+e^{4\cosh^{-1}\left(\frac{\epsilon_{DS}+\epsilon}{\Delta}\right)}+1}+2\right)+$$
$$-\left(f^+_{\mathrm{S_R}}(\epsilon)-f^-_{\mathrm{S_L}}(\epsilon)\right)\frac{\left(e^{2\cosh^{-1}\left(\frac{\epsilon_{DS}+\epsilon}{\Delta}\right)}-1\right)^2}{-2e^{2\cosh^{-1}\left(\frac{\epsilon_{DS}+\epsilon}{\Delta}\right)}\cos\left(\frac{2\epsilon_{DS}}{\epsilon_C}+\frac{2L(\epsilon_{DS}+\epsilon)}{\Delta}+\phi\right)+e^{4\cosh^{-1}\left(\frac{\epsilon_{DS}+\epsilon}{\Delta}\right)}+1}+$$
$$\left.-\left(f^+_{\mathrm{S_L}}(\epsilon)-f^-_{\mathrm{S_R}}(\epsilon)\right)\frac{\left(e^{2\cosh^{-1}\left(\frac{\epsilon-\epsilon_{DS}}{\Delta}\right)}-1\right)^2}{-2e^{2\cosh^{-1}\left(\frac{\epsilon-\epsilon_{DS}}{\Delta}\right)}\cos\left(-\frac{2\epsilon_{DS}}{\epsilon_C}+\frac{2L(\epsilon-\epsilon_{DS})}{\Delta}-\phi\right)+e^{4\cosh^{-1}\left(\frac{\epsilon-\epsilon_{DS}}{\Delta}\right)}+1}\right]|t|^2+\mathcal{O}(|t|^4) \tag{S.14}$$

$$j^0_{N,IV}\equiv j^0_{N,III} \tag{S.15}$$

Here we consider the Fermi functions $f^\alpha_j(\epsilon)=\{\exp[(\epsilon-\alpha\mu_j)/k_BT_j)]+1\}^{-1}$ of the leads $j=\mathrm{S_L},\mathrm{S_R},\mathrm{N}$ with $\mu_N=eV_N$ and $\mu_{\mathrm{S_R}}=\mu_{\mathrm{S_R}}=0$ (i.e. superconductors are grounded); in the case in which the leads have independent temperatures $T_\mathrm{N},T_{\mathrm{S_L}},T_{\mathrm{S_R}}$ with $T_N\lesssim\min\left(T_{\mathrm{S_L}},T_{\mathrm{S_R}}\right)$, so that the heat flow between the probe and the TI does not affect neither the superconducting state of the contacts nor the proximization with the TI. It is interesting to discuss some important experimental consequences which can be immediately derived by looking the previous expressions. We observe that the current integrands are factorized in terms of the Fermi function differences $f^+_N(\epsilon)-f^-_N(\epsilon)$ and $f^\pm_{\mathrm{S_L}}(\epsilon)-f^\mp_{\mathrm{S_R}}(\epsilon)$. Notably, it can be shown that this happens not only in the opaque limit, but for every coupling with the probe (here we do not report the analytical expressions for brevity). As a consequence of this, there is no contribution from the Fermi function of the normal probe when $V_N=0$ since $f^+_N(\epsilon)=f^-_N(\epsilon)$. This clearly shows that, even in the non-linear regime, there is no thermoelectrical contribution induced by any thermal gradient between the probe and the TI edge since the probe temperature does not even appear in the expressions. It is important to stress that this implies that the charge current in the normal probe does not depend on exact value of $T_N$. In the main text we have considered $T_N=T$ just for convenience. The only contribution to the thermoelectric current in the probe, instead, is purely nonlocal due to the application of a thermal gradient $\delta T=T_{\mathrm{S_L}}-T_{\mathrm{S_R}}$ between the two superconductors; in which case the Fermi function differences $f^\pm_{\mathrm{S_L}}(\epsilon)-f^\mp_{\mathrm{S_R}}(\epsilon)$ are not zero.

## COMPARISON WITH THE TUNNELING APPROACH

In this section we compare the results obtained using the scattering approach with the results obtained using the tunneling approach [1–3]. For the latter we use the formulation presented in Ref. [2], but modifying the density of

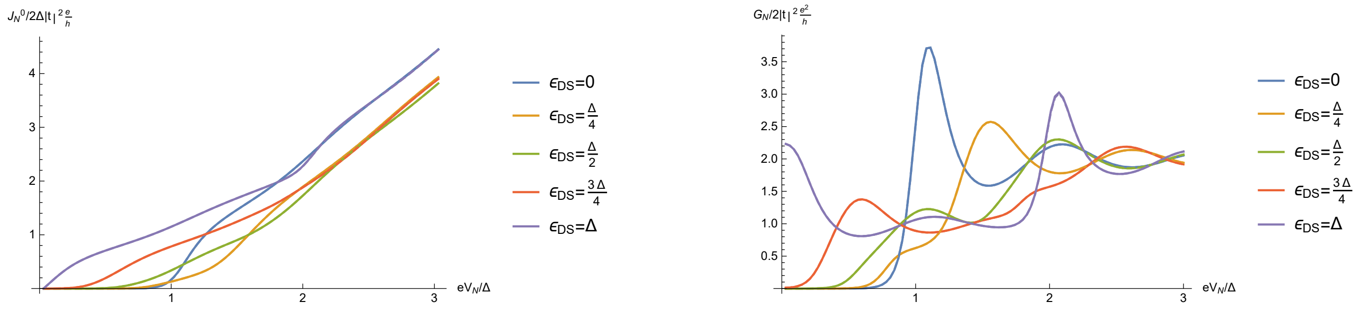


(a) (b)

Figure 2: (a) - The charge current $J_N^0$ at the metallic probe. Scattering results (solid lines) coincide with the tunneling ones (dashed lines), curves overlap. (b) - The differential conductance $G_N$ at the metallic probe. Scattering results (solid lines) coincide with the tunneling ones (dashed lines), curves overlap. In both the plots we considered $L/\xi = 3$, $T/T_C = 1/10$ and $\phi = 0$.

states (DOS) [Eq. (14)] by adding an imaginary part $\gamma$ to the energy in order to phenomenologically capture the contribution of Andreev bound states. Regarding the scattering approach we consider the expression of the current $J_N^0$ at lowest order in $|t|^2$ derived in the previous section. In Figs. 2(a) and 2(b) we plot the current $J_N^0$ and the differential conductance $G_N = dJ_N^0/dV_N$, respectively, as functions of the electrochemical potential $eV_N$ for different values of $\epsilon_{\rm DS}$ and setting $\gamma = 0$. As expected, on the scale of the plot the curves relative to the two approaches coincide for both quantities. The density plot of the differential conductance $G_N$ is also shown in Figs. 3(a) and 3(b) for the two approaches, respectively, as a function of $eV_N$ and $\epsilon_{\rm DS}$. Again, we see that the conductance $G_N$ in the two approaches always coincides.

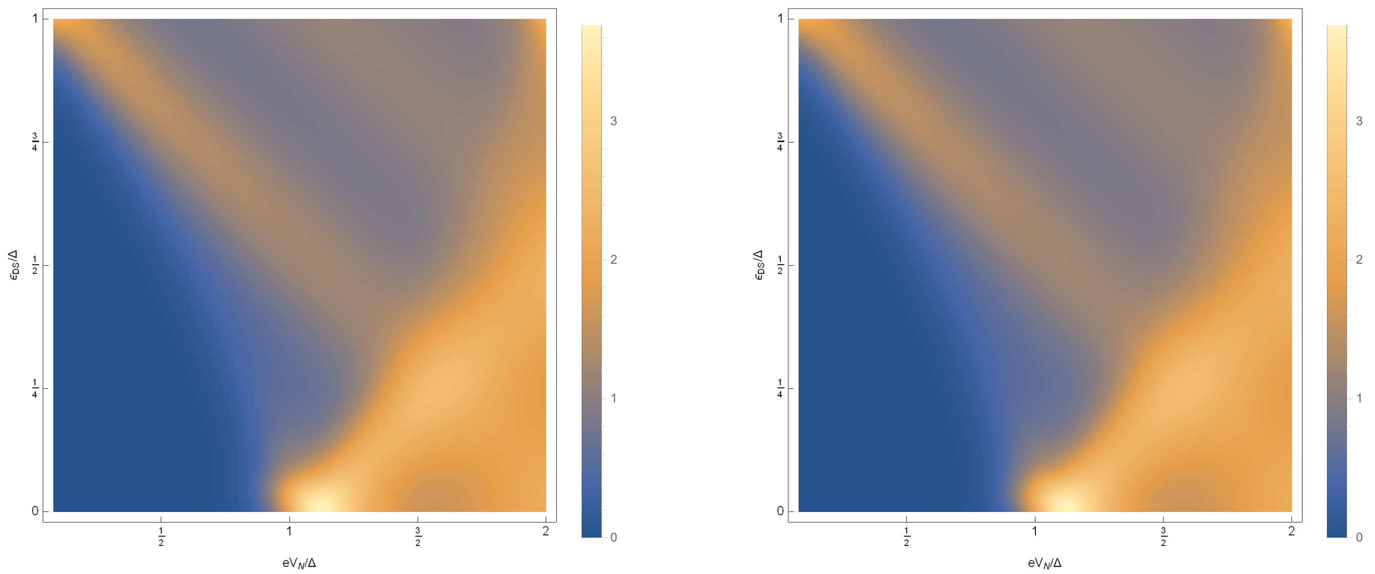


(a) (b)

Figure 3: (a) - Density plot of the differential conductivity $G_N$ at the metallic probe obtained with the scattering approach in the leading order in $t$. (b) - Density plot of the differential conductivity $G_N$ at the metallic probe obtained with the tunneling approach with $\gamma = 0$. In both the plots we considered $L/\xi = 3$, $T/T_C = 1/10$ and $\phi = 0$.

It is now important to notice that the expression for the current $J_N^0$ in the scattering approach at lowest order in $|t|^2$ do not describe the results of the tunneling approach when a finite value of $\gamma$ is taken. Indeed, in such a case $G_N$ presents additional features produced by the ABSs [see Fig. 4(b), to be compared with Fig. 3(a)]. This is expected because ABSs are accounted for by the scattering approach at the order $\mathcal{O}\left(|t|^4\right)$. By using the exact scattering approach one obtains the results reported in Fig. 4(a) for $|t|^2 = 10^{-2}$. By comparing the two panels of Fig. 4, we see

that they show qualitatively the same behavior (highlighting the presence of the ABSs in the same positions inside the gap), but they do not exactly match. The difference is due to the effective description of the tunneling approach with respect to the exact scattering approach.

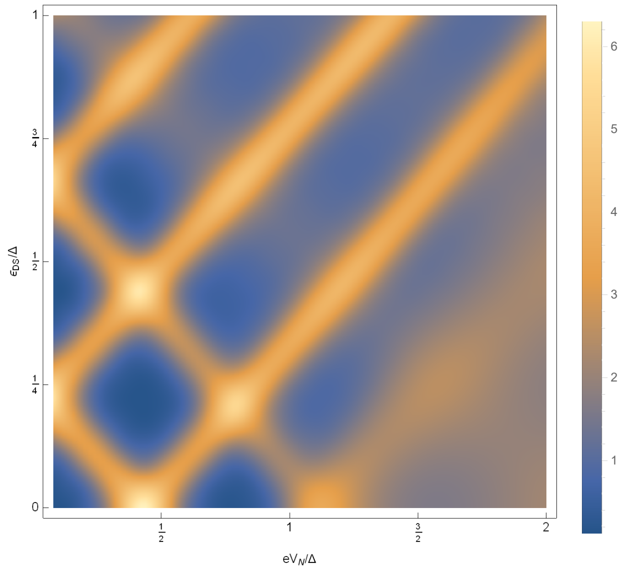


(a)

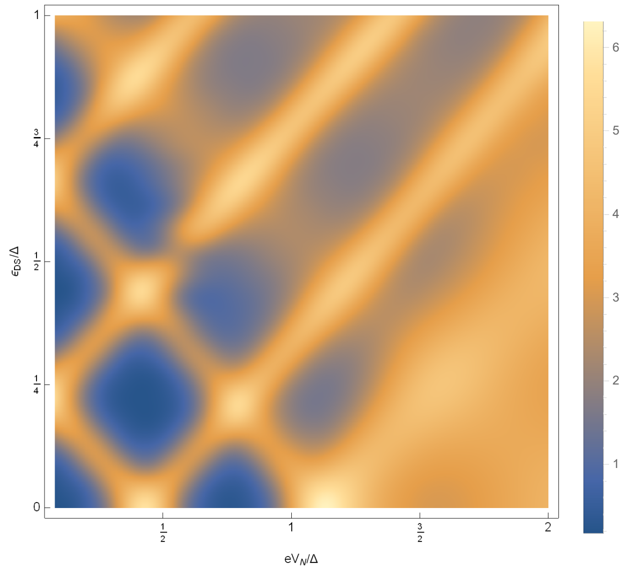


(b)

Figure 4: (a) - Density plot of the differential conductance obtained in the scattering approach. $G_N$ is normalized with respect to the transmittance of the probe $|t|^2 = 10^{-2}$. (b) - Density plot of the differential conductance obtained in the tunneling approach. Here $\gamma = \frac{\Delta}{100}$. In both the plots we considered $L/\xi = 3$, $T/T_C = 1/10$ and $\phi = 0$.

A more direct comparison between tunneling approach and exact scattering approach is given in Fig. 5 where the linear-response conductance $\sigma = L_{11}/T$ is plotted as a function of $\epsilon_{\mathrm{DS}}$ for various values of $\phi$. The two approaches almost exactly coincide apart from a dip in the peak at $\phi = 0$ present in the tunneling curve (green dashed line).

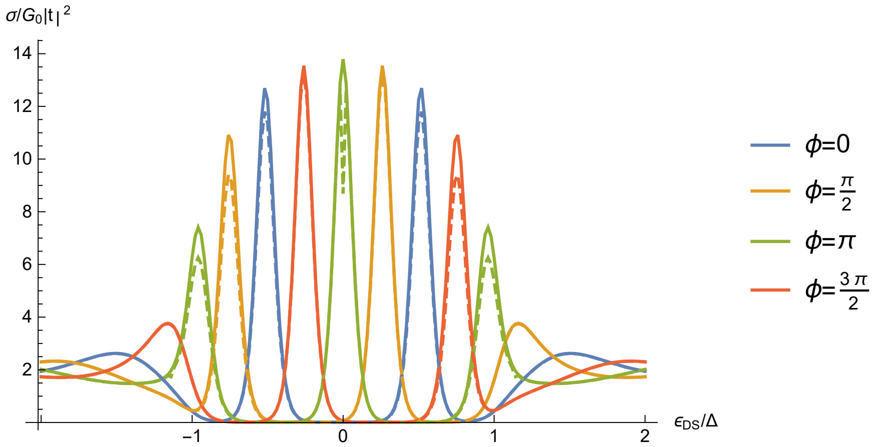


Figure 5: Linear regime - Scattering-Tunneling Comparison - Electrical conductance $\sigma$ in units of $G_0|t|^2$ (with $G_0 = \frac{2e^2}{h}$ the electrical conductance quantum), as a function of $\epsilon_{DS}/\Delta$. Different curves refer to different values of the phase difference $\phi$ between the two superconductors. Solid lines for the scattering approach (specifically $|t|^2 = 10^{-2}$), dashed lines for the tunneling approach ($\gamma = \frac{\Delta}{1000}$). The other parameters are: $L/\xi = 3$, $T/T_C = 1/10$ and $\phi = 0$.

We conclude the discussion by noting that only applying the full scattering formalism one can have a complete and consistent description of the transport in the three terminal setup which fully include the influence of ABSs. Similar considerations can be applied to the thermoelectrical current in the probe. In particular, we find that the scattering formalism shows, as naively expected, that ABSs do not contribute neither to thermal or to thermoelectrical current

in the probe. One can analytically show that, at $V_N = 0$, there is no contribution to the N probe thermoelectric current from ABSs for arbitrary values of $|t|^2$.

## THERMAL CONDUCTANCE WITHOUT THE PROBE

In this section is presented the thermal conductance $\kappa = L_{22}/T^2$ calculated with the scattering approach by uncoupling the probe (i. e. setting $t = 0$) and compared with the results presented in Ref. [4] calculated using the DOS. As expected the two approaches are completely equivalent: curves overlap for all the parameters - see Fig. 6.

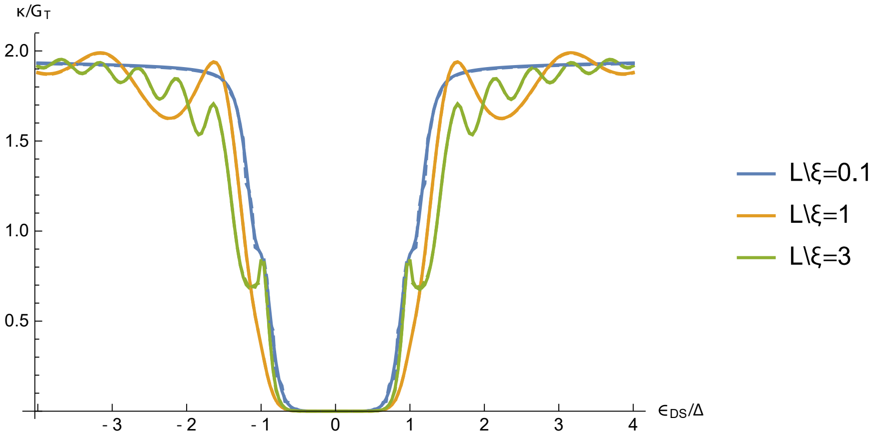


Figure 6: Linear regime - Comparison between the scattering approach (without the probe) and the DOS method presented in Ref. [4] - Thermal conductance $\kappa$ in units of the thermal conductance quantum $G_T = \frac{\pi^2}{3h} k_B^2 T$, as a function of $\epsilon_{DS}/\Delta$. Different curves refer to different values of $L/\xi = 1/10, 1, 3$. Solid lines for the scattering approach, dashed lines for the results obtained using the DOS [4]: curves exactly overlap. Other parameters: $T/T_C = 1/10$ and $\phi = 0$.

## THERMOELECTRIC FIGURE OF MERIT ZT

Here we show the figure of merit $ZT$ which parametrizes the maximum achievable efficiency $\eta^{max} = \eta_C \frac{\sqrt{ZT+1}-1}{\sqrt{ZT+1}+1}$ (which approaches to the Carnot efficiency $\eta_C = \delta T/T$ for $ZT \to \infty$) in the linear regime when the device is regarded as a thermoelectric heat-engine/refrigerator. In our case this is defined as

$$ZT = -\frac{L_{12}L_{21}}{L_{11}L_{22}}, \tag{S.16}$$

since $L_{12} = -L_{21}$. We plot $ZT$ in Fig. 7 as a function of $\epsilon_{DS}$ and $|t|^2$ for the parameters specified in the caption. Notice that the value of $ZT$ achieves its highest value at $\epsilon_{DS} \sim \pm\Delta$ (where the Seebeck is maximal). Interestingly, $ZT$ is maximal for $|t|^2 = 1$, i.e. in the regime of maximum coupling with the probe, but reaching quite small values $\sim 0.1$. In this respect we notice that a coupling with the normal probe containing an additional energy filter like a quantum dot would lead to higher values. As a final remark, we notice that the $ZT$ and the Seebeck coefficient $S$ present opposite behaviors as functions of coupling parameter $|t|^2$. More specifically the Seebeck coefficient takes higher values in the weak coupling limit ($|t|^2$ small), while $ZT$ is largest in the strong coupling limit ($|t|^2$ close to 1). First we notice that, in general the Seebeck coefficient $S$ and the figure of merit $ZT$ are not expected to have the same behavior. Being more specific, in our system (similarly to the standard case of ordinary two-terminal systems), this can be understood by rewriting Eq. (S.16) as $\mathrm{ZT} = S^2 T^2 \frac{L_{11}}{L_{22}}$, where we explicitly see that $ZT$ does not only depend on $S$ but also on the quotient between the electrical ($\propto L_{11}$) and thermal ($\propto L_{22}$) conductances. The behavior of the corresponding Onsager coefficients is shown in Fig. 2 as functions of $|t|^2$, while $S$ is shown in Fig.3 of the main text. For clarity we will fix $\epsilon_{\mathrm{DS}}/\Delta \simeq \pm 1$ where the Seebeck coefficient is maximal. We can see that $S$ increases as $|t|^2$ decreases, while $\frac{L_{11}}{L_{22}}$ gets suppressed for $|t|^2 \to 0$, since $L_{22}$ in the denominator tends to a constant [see Fig.2 (b) of the main text], while $L_{11}$ in the numerator goes to zero (due to the decoupling with the probe). As a consequence,

$ZT$ tends to zero in the weak coupling limit. In the strong coupling limit ($|t|^2 \to 1$), $S$ goes to a constant, while $L_{11}$ increases and $L_{22}$ decreases [see Fig. 2(b) and (c) of the main text], resulting in an overall increase of the $ZT$.

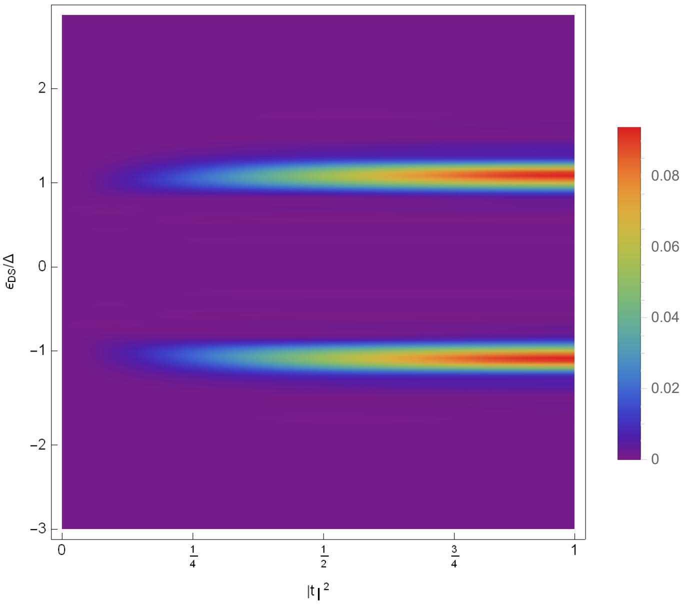


Figure 7: Density plot of the figure of merit $ZT$ plotted as a function of $\epsilon_{DS}/\Delta$ and $|t|^2$. The parameters used are: $L/\xi = 1$, $T/T_C = 1/10$ and $\phi = 0$.

## DEPENDENCE ON THE JUNCTION LENGTH $L$

In the main text we discussed the case in which the length of the junction is equal to the coherence length of the system, i. e. $L = \xi$. For our setup, this situation is reasonable assuming a STM tip with state-of-the-art size of 100 nm and a coherence length $\xi$ in the proximized TI of the order of 600 nm [8, 9]. Further a length $L \sim \xi$ assures that the transport along the edge state is ballistic [14] at the operating temperatures for our the setup, typically of a few K. In this section we complete the analysis by investigating the behavior of the Onsager coefficients $L_{ij}$ as functions of $\epsilon_{DS}(\Phi)/\Delta$ and the coupling parameter $|t|^2$ for short ($L/\xi = 0.1$, Fig. 8) and long ($L/\xi = 5$, Fig. 9) junctions. By comparing Figs. 8 and 9 with Fig. 2 in the main text, it is easy to see that the main result of our paper (namely, the occurrence of a purely non-local thermoelectric current due to the helical nature of the edge states) is not modified. In particular, when the gap closes due to the flux bias $\Phi$, i.e. when $|\epsilon_{DS}(\Phi)/\Delta| \approx 1$, the non-local thermoelectric current is maximized *for any length*. For long junctions the only additional feature is the presence of oscillations in the linear-response coefficients, due to the proliferation of resonant states in the junction (see Fig. 9). No oscillations occur, though, at any lengths when $|t|^2 \approx 1$.

## THERMOELECTRIC CURRENT FOR A PROXIMIZED 2D TI

In this section we apply our results to the case of a 2D TI made of HgTe/HgCdTe quantum wells, proximized with Aluminium with a induced gap $\Delta \approx 40\,\mu\text{eV}$ (see Ref. [10]). More precisely, we compute the non-local thermoelectric current $J_{12} = J_1^0|_{V_N=0}$, defined as the charge current at the probe when $V_N = 0$. We assume a bad (ohmic) contact with the probe (namely $|t|^2 \approx 0.1$) and a thermal gradient of the order of 80-120 mK, a realistic value for these type of experimental setups [6]. In Fig. 10 we depict the thermoelectric current $J_{12}$ as a function of the flux bias $\Phi$ and the temperature gradient $\delta T \lesssim 120\,\text{mK}$, such that the induced gap of the right and left proximized regions are constant and equal to $\Delta$. Fig. 10 [main panel and inset (b)] shows that when the gap closes by tuning the flux bias $\Phi$ such that $|\epsilon_{DS}(\Phi)/\Delta| \approx 1$, the non-local thermoelectric current is maximal, reaching values of the order $\approx 30\,\text{pA}$ (a reasonable value for these kind of experiments [8]). Moreover, we notice that, as shown in the inset $(a)$ of Fig. 10, the current has a linear behavior in $\delta T$ up to 80 mK. As a final remark, we notice that the specific choice of paramenters we have just

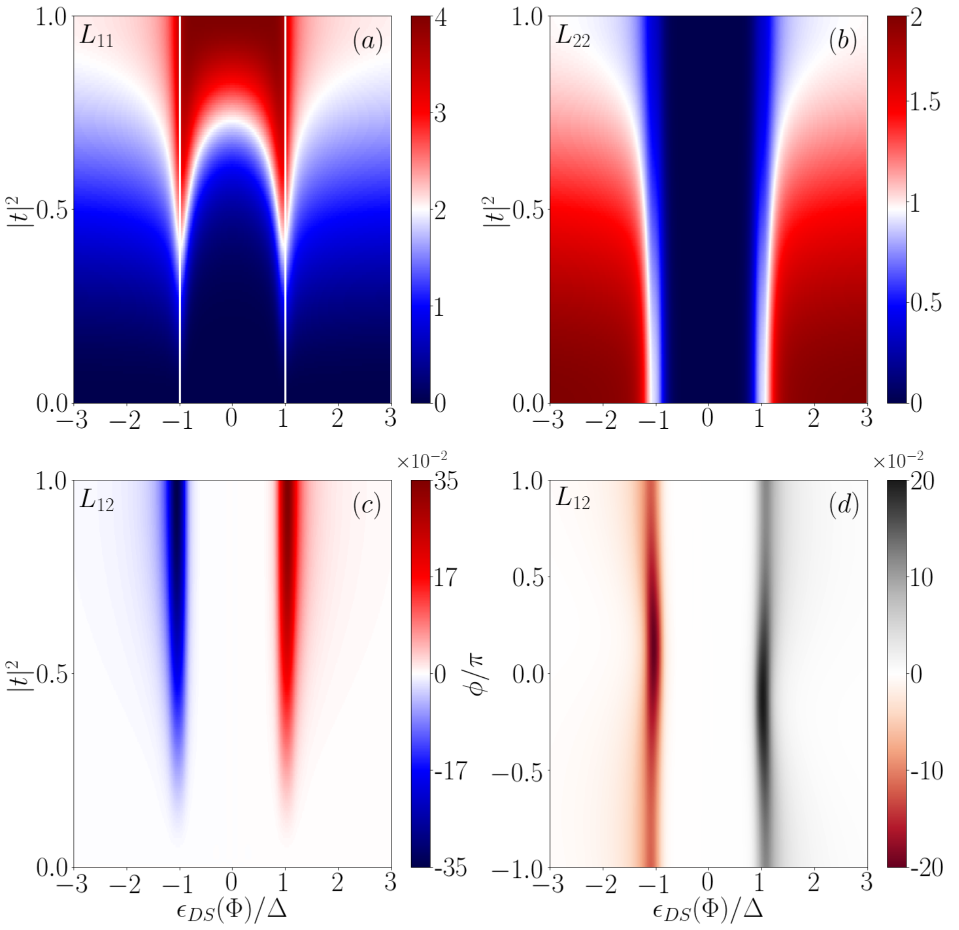


Figure 8: Onsager coefficients $L_{11}$ (a), $L_{22}$ (b) and $L_{12} = -L_{21}$ (c) in the case of short junction $L/\xi = 0.1$, as functions of $\epsilon_{DS}(\Phi)/\Delta$ and the coupling parameter $|t|^2$ for phase bias $\phi = \phi_{S_L} - \phi_{S_R} = 0$, $T/T_C = 0.1$ and $L/\xi = 1$. (d) $L_{12}$ as a function of $\epsilon_{DS}(\Phi)/\Delta$ and the phase difference $\phi$ for $|t|^2 = 0.5$. Such quantities are normalized as follows: $L_{11}/(G_0 T)$, $L_{22}/(G_T T^2)$ and $L_{12}/(\sqrt{G_0 G_T T^3})$.

discussed is not optimal. Indeed, we stress that much higher values of the current and larger operation temperatures can be obtained with different materials [11–13] or fully proximized structures, i. e. when the induced gap in the 2D TI is equal to the $\Delta$ of the superconductor.


* Electronic address: gianmichele.blasi@sns.it
† Electronic address: alessandro.braggio@nano.cnr.it



[1] B. Sothmann and E. M. Hankiewicz, Phys. Rev. B **94**, 081407 (R), (2016).
[2] L. Bours, B. Sothmann, M. Carrega, E. Strambini, E. M. Hankiewicz, L. W. Molenkamp, and F. Giazotto, Phys. Rev. Applied **10**, 014027 (2018).
[3] L. Bours, B. Sothmann, M. Carrega, E. Strambini, A. Braggio, E. M. Hankiewicz, L. W. Molenkamp, and F. Giazotto, Phys. Rev. Applied **11** 044073 (2019).
[4] B. Sothmann, F. Giazotto and E. M. Hankiewicz, New J. Phys. **19** 023056 (2017).
[5] C. J. Lambert and R. Raimondi, J. Phys. Condens. Matter **10**, 901 (1998)
[6] F. Giazotto, T. T. Heikkilä, A. Luukanen, A. M. Savin, and J. P. Pekola Rev. Mod. Phys. **78**, 217 (2009)
[7] L. Lunczer, P. Leubner, M. Endres, V. L. Müller, C. Brüne, H. Buhmann, and L. W. Molenkamp, Phys. Rev. Lett. 123, 047701 (2019)
[8] S. Hart, H. Ren, T. Wagner, P. Leubner, M. Mühlbauer, C. Brüne, H. Buhmann, L. W. Molenkamp and A. Yacoby Nature Phys. **10**, 638 (2014).
[9] E. Bocquillon, R. S. Deacon, J. Wiedenmann, P. Leubner, T. M. Klapwijk, C. Brüne, K. Ishibashi, H. Buhmann, and L.

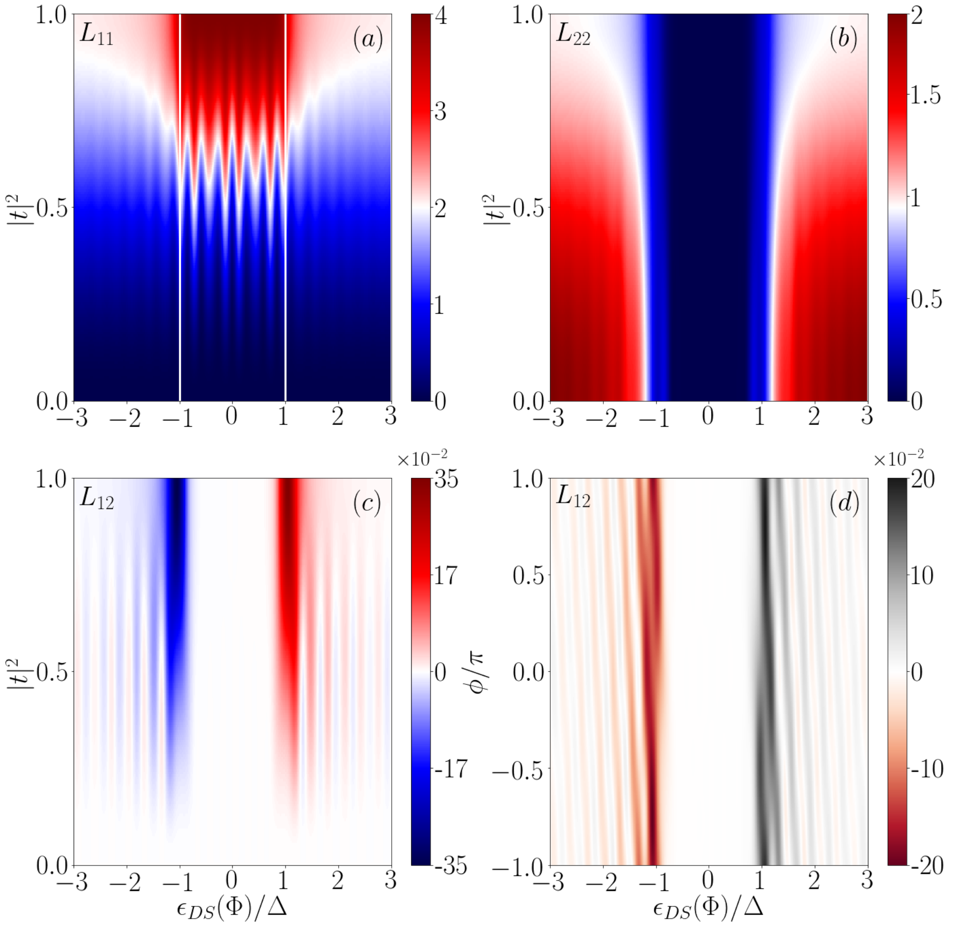


Figure 9: Onsager coefficients $L_{11}$ (a), $L_{22}$ (b) and $L_{12} = -L_{21}$ (c) in the case of long junction $L/\xi = 5$, as functions of $\epsilon_{DS}(\Phi)/\Delta$ and the coupling parameter $|t|^2$ for phase bias $\phi = \phi_{S_L} - \phi_{S_R} = 0$, $T/T_C = 0.1$ and $L/\xi = 1$. (d) $L_{12}$ as a function of $\epsilon_{DS}(\Phi)/\Delta$ and the phase difference $\phi$ for $|t|^2 = 0.5$. Such quantities are normalized as follows: $L_{11}/(G_0 T)$, $L_{22}/(G_T T^2)$ and $L_{12}/(\sqrt{G_0 G_T T^3})$.


W. Molenkamp, Nature Nanotech. **12**, 137 (2017).

[10] E. Bocquillon, J. Wiedenmann, R. S. Deacon, T. M. Klapwijk, H. Buhmann, L. W. Molenkamp (2018) *Topological Matter*. Springer, Cham.

[11] G. Tkachov. *Topological insulators: The physics of spin helicity in quantum transport*. Pan Stanford, 2015.

[12] B. A. Bernevig, T. L. Hughes. *Topological insulators and topological superconductors*. Princeton university press, 2013.

[13] M. Franz, L. Molenkamp. *Topological Insulators*. Elsevier, 2013.

[14] S. Groenendijk, G. Dolcetto, and T. L. Schmidt, Phys. Rev. B **97**, 241406 (2018)

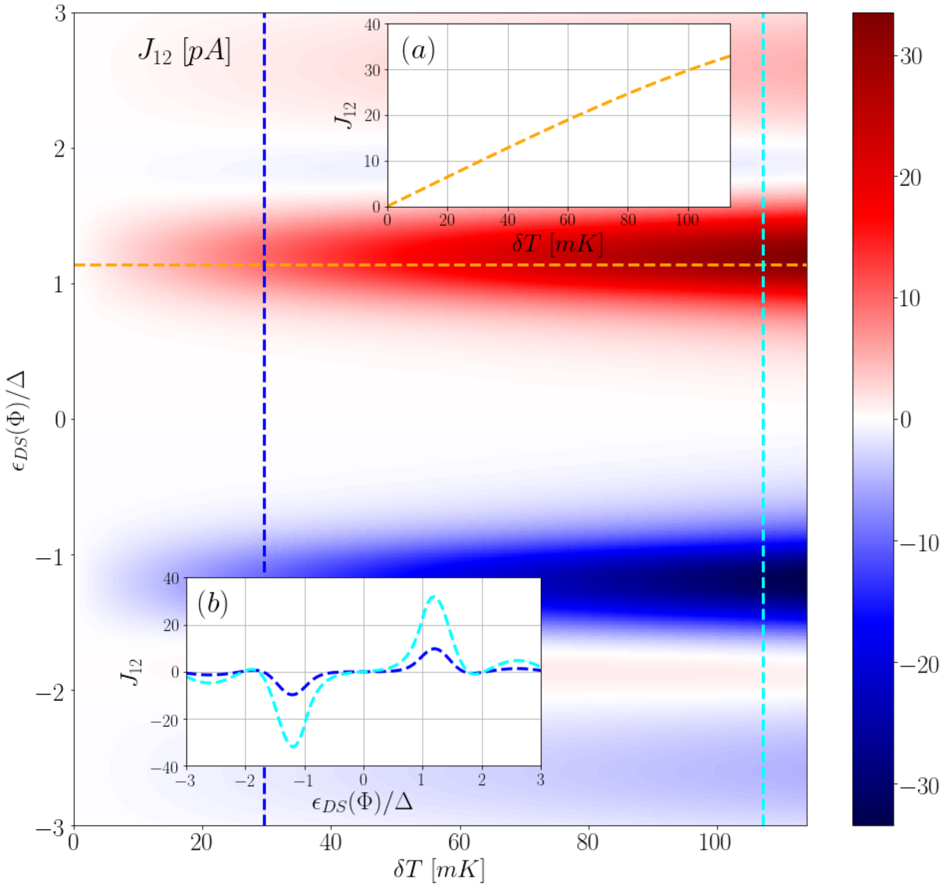


Figure 10: Density plot of the thermoelectric current $J_{12}$ expressed in $pA$, as function of $\epsilon_{DS}(\Phi)/\Delta$ and the thermal gradient $\delta T$ expressed in units of mK, for phase bias $\phi = \phi_{\mathrm{S_L}} - \phi_{\mathrm{S_R}} = 0$, $L/\xi = 1$ and $|t|^2 = 0.1$. In the inset $(a)$ is depicted the behavior of $J_{12}$ as a function of $\delta T$ corresponding to an horizontal cut at $\epsilon_{DS}(\Phi)/\Delta \approx 1$ (orange dashed line). In the inset $(b)$ is depicted the behavior of $J_{12}$ as a function of $\epsilon_{DS}(\Phi)/\Delta$ corresponding to vertical cuts at $\delta T = 30\,\mathrm{mK}, 110\,\mathrm{mK}$ (dark and light blue dashed lines).
